# Supplementary material for: Fairness at Every Intersection: Uncovering and Mitigating Intersectional Biases in Multimodal Clinical Predictions
Source: arXiv:2412.00606 source file (2026-09-18)
Supplement: Supplementary file 1 [file supplementary.tex]

%File: anonymous-submission-latex-2025.tex
\documentclass[letterpaper]{article} % DO NOT CHANGE THIS
\usepackage[submission]{aaai25}  % DO NOT CHANGE THIS
\usepackage{times}  % DO NOT CHANGE THIS
\usepackage{helvet}  % DO NOT CHANGE THIS
\usepackage{courier}  % DO NOT CHANGE THIS
\usepackage[hyphens]{url}  % DO NOT CHANGE THIS
\usepackage{graphicx} % DO NOT CHANGE THIS
\urlstyle{rm} % DO NOT CHANGE THIS
  % DO NOT CHANGE THIS
\usepackage{natbib}  % DO NOT CHANGE THIS AND DO NOT ADD ANY OPTIONS TO IT
\usepackage{caption} % DO NOT CHANGE THIS AND DO NOT ADD ANY OPTIONS TO IT
\frenchspacing  % DO NOT CHANGE THIS
\setlength{\pdfpagewidth}{8.5in} % DO NOT CHANGE THIS
\setlength{\pdfpageheight}{11in} % DO NOT CHANGE THIS
%
% These are recommended to typeset algorithms but not required. See the subsubsection on algorithms. Remove them if you don't have algorithms in your paper.
\usepackage{algorithm}
\usepackage{algorithmic}

\usepackage{booktabs}%
\usepackage{amsmath,amssymb,amsfonts,amsthm}%
\usepackage{todonotes}
\usepackage{pifont}

\usepackage[submission]{aaai25}  % DO NOT CHANGE THIS
\usepackage{times}  % DO NOT CHANGE THIS
\usepackage{helvet}  % DO NOT CHANGE THIS
\usepackage{courier}  % DO NOT CHANGE THIS
\usepackage[hyphens]{url}  % DO NOT CHANGE THIS
\usepackage{graphicx} % DO NOT CHANGE THIS
\urlstyle{rm} % DO NOT CHANGE THIS
  % DO NOT CHANGE THIS
\usepackage{natbib}  % DO NOT CHANGE THIS AND DO NOT ADD ANY OPTIONS TO IT
\usepackage{caption} % DO NOT CHANGE THIS AND DO NOT ADD ANY OPTIONS TO IT
\frenchspacing  % DO NOT CHANGE THIS
\setlength{\pdfpagewidth}{8.5in} % DO NOT CHANGE THIS
\setlength{\pdfpageheight}{11in} % DO NOT CHANGE THIS
%
% These are recommended to typeset algorithms but not required. See the subsubsection on algorithms. Remove them if you don't have algorithms in your paper.
\usepackage{algorithm}
\usepackage{algorithmic}

\usepackage{booktabs}%
\usepackage{amsmath,amssymb,amsfonts}%
\usepackage{todonotes}
\usepackage{pifont}
\usepackage{times}
\usepackage{graphicx}
\usepackage{subcaption}
\usepackage{colortbl}
\usepackage{array}
\usepackage[T1]{fontenc}
\usepackage[utf8]{inputenc}
\usepackage{microtype}
\usepackage{inconsolata}
\usepackage{enumitem}
\usepackage{caption}
\setlength{\pdfpagewidth}{8.5in} % DO NOT CHANGE THIS
\setlength{\pdfpageheight}{11in} % DO NOT CHANGE THIS
\usepackage{algorithm}
\usepackage{algorithmic}

\usepackage{booktabs}%
\usepackage{amsmath,amssymb,amsfonts,amsthm}%
\usepackage{todonotes}
\usepackage{pifont}

%
% These are are recommended to typeset listings but not required. See the subsubsection on listing. Remove this block if you don't have listings in your paper.
\usepackage{newfloat}
\usepackage{listings}
\DeclareCaptionStyle{ruled}{labelfont=normalfont,labelsep=colon,strut=off} % DO NOT CHANGE THIS
\lstset{%
	basicstyle={\footnotesize\ttfamily},% footnotesize acceptable for monospace
	numbers=left,numberstyle=\footnotesize,xleftmargin=2em,% show line numbers, remove this entire line if you don't want the numbers.
	aboveskip=0pt,belowskip=0pt,%
	showstringspaces=false,tabsize=2,breaklines=true}
\floatstyle{ruled}
\newfloat{listing}{tb}{lst}{}
\floatname{listing}{Listing}
%

%
% These are are recommended to typeset listings but not required. See the subsubsection on listing. Remove this block if you don't have listings in your paper.
\usepackage{newfloat}
\usepackage{listings}
\DeclareCaptionStyle{ruled}{labelfont=normalfont,labelsep=colon,strut=off} % DO NOT CHANGE THIS
\lstset{%
	basicstyle={\footnotesize\ttfamily},% footnotesize acceptable for monospace
	numbers=left,numberstyle=\footnotesize,xleftmargin=2em,% show line numbers, remove this entire line if you don't want the numbers.
	aboveskip=0pt,belowskip=0pt,%
	showstringspaces=false,tabsize=2,breaklines=true}
\floatstyle{ruled}
\newfloat{listing}{tb}{lst}{}
\floatname{listing}{Listing}
%
% Keep the \pdfinfo as shown here. There's no need
% for you to add the /Title and /Author tags.
\pdfinfo{
/TemplateVersion (2025.1)
}

\setcounter{secnumdepth}{2} %May be changed to 1 or 2 if section numbers are desired.

% The file aaai25.sty is the style file for AAAI Press
% proceedings, working notes, and technical reports.
%

% Title

% Your title must be in mixed case, not sentence case.
% That means all verbs (including short verbs like be, is, using,and go),
% nouns, adverbs, adjectives should be capitalized, including both words in hyphenated terms, while
% articles, conjunctions, and prepositions are lower case unless they
% directly follow a colon or long dash
\title{Supplementary Materials: \\Fairness at Every Intersection: Uncovering and Mitigating Intersectional Biases in Multimodal Clinical Predictions }
\author{
    %Authors
    % All authors must be in the same font size and format.
    \textsuperscript{\rm 1},
    \textsuperscript{\rm 2},
    \textsuperscript{\rm 1}, and
    \textsuperscript{\rm 1}
}
\affiliations{
    %Afiliations
    \textsuperscript{\rm 1}Department of Computer and Information Science (IDA), Link\"oping University, Sweden\\
	 \textsuperscript{\rm 2}Institute for Experiential AI, Northeastern University, USA\\
	 md.fahim.sikder@liu.se, r.ramachandranpillai@northeastern.edu, \\ \{daniel.de.leng, fredrik.heintz\}@liu.se
%
% See more examples next
}

%Example, Single Author, ->> remove \iffalse,\fi and place them surrounding AAAI title to use it
% \iffalse
% \title{Generating Synthetic Fair Syntax-agnostic Data by Learning and Distilling Fair Representation}
% \author {
%     Author Name
% }
% \affiliations{
%     Affiliation\\
%     Affiliation Line 2\\
%     name@example.com
% }
% \fi

% \iffalse
% %Example, Multiple Authors, ->> remove \iffalse,\fi and place them surrounding AAAI title to use it
% \title{My Publication Title --- Multiple Authors}
% \author {
%     % Authors
%     First Author Name\textsuperscript{\rm 1},
%     Second Author Name\textsuperscript{\rm 2},
%     Third Author Name\textsuperscript{\rm 1}
% }
% \affiliations {
%     % Affiliations
%     \textsuperscript{\rm 1}Affiliation 1\\
%     \textsuperscript{\rm 2}Affiliation 2\\
%     firstAuthor@affiliation1.com, secondAuthor@affilation2.com, thirdAuthor@affiliation1.com
% }
% \fi

% REMOVE THIS: bibentry
% This is only needed to show inline citations in the guidelines document. You should not need it and can safely delete it.
\usepackage{bibentry}
% END REMOVE bibentry

\begin{document}

\maketitle

\section{Workflow}
Figure 1 shows the overall flowchart of the proposed method. It starts with learning a unified textual representation from all the available modalities and then employs pre-trained clinical language embeddings to learn the interoperability of features. Finally, sub-group-specific multimodal classifiers are built on the dataset split and do customized voting to exploit the disagreement region. 

\begin{figure*}[hbt!]
    \centering
    \includegraphics[width=0.7\textwidth,height=5cm]{Fig/image (49).png} 
    \caption{The overall workflow}
    \label{fig:example}
\end{figure*}
\section{Dataset Statistics}
\label{sec:Data}

\begin{table*}[hbt!]
\centering
\small
\begin{tabular}{cccccc}
\toprule
\textbf{Gender} & \multicolumn{4}{c|}{\textbf{Race}} & \textbf{Total} \\
% \cmidrule{2-5}
 & \textbf{White} & \textbf{Black} & \textbf{Other} & \textbf{Asian} & \\
\midrule
Male & 4153 (26.58\%) & 2093 (13.39\%) & 1025 (6.56\%) & 219 (1.4\%) & 7490 (47.93\%) \\
Female & 4435 (28.38\%) & 2596 (16.61\%) & 866 (5.54\%) & 240 (1.54\%) & 8137 (52.07\%)  \\

\textbf{Total} & 8588 (54.96\%) & 4689 (30.00\%) & 1891 (12.10\%) & 459 (2.94\%) & 15627 (100.00\%) \\
\bottomrule
\end{tabular}
\caption{ Distribution of Stay IDs and subgroup statistics in MIMIC-eye}
\label{tab:counts}
\end{table*}

\begin{table*}[hbt!]
\centering
\small
\begin{tabular}{cccc}
\toprule
\textbf{Gender} & \multicolumn{2}{c|}{\textbf{Race}} & \textbf{Total} \\
% \cmidrule{2-3}
 & \textbf{White} & \textbf{Non-White} & \\
\midrule
Male & 112606 (28.15\%) & 70209 (17.55\%) & 182815 (45.70\%) \\
Female & 120639 (30.16\%) & 96565 (24.14\%) & 217204 (54.30\%)  \\

\textbf{Total} & 233245 (58.31\%) & 166774 (41.69\%) & 400019 (100\%) \\
\bottomrule
\end{tabular}
\caption{Distribution of Stay IDs and subgroup statistics in MIMIC-IV-ED}
\label{tab:counts}
\end{table*}

MIMIC-IV-ED is a public database of emergency department (ED) admissions at the Beth Israel Deaconess Medical Center between 2011 and 2019. The database contains vital signs, triage information, medication administration, and discharge diagnosis information for about 400,000 ED stays.
 
The MIMIC-Eye dataset (Hsieh et al. 2023)4 integrates various datasets associated with the Medical Information Mart for Intensive Care (MIMIC), offering a comprehensive collection of patient information. It includes medical images such as chest X-rays (available in both MIMIC CXR and MIMIC JPG formats), clinical data from the MIMIC IV Emergency Department (ED), detailed patient hospital journey records from MIMIC IV, and eye-tracking data capturing gaze information and pupil dilations.
 
The MIMIC-Eye dataset consists of records from 3,192 patients, encompassing 3,689 chest X-ray images linked to various modalities. Each patient’s data includes multiple stay-ids, amounting to over 15627 stay-ids in total. Each patient’s record contains information on lab events, medical details, chest X-rays, and their corresponding reports. Table \ref{tab:counts} shows the distribution of Stay IDs broken down by various sensitive subgroups and \ref{tab:reduced-directory-structure} shows the metadata.

%This dataset consists of records from 3,192 patients, encompassing 3,689 chest X-ray images linked to various modalities. Each patient's data includes multiple stay-ids, amounting to over 15627 stay-ids in total. Each patient's record contains information on lab events, medical details, chest X-rays, and their corresponding reports. Table \ref{tab:counts} shows the distribution of Stay IDs broken down by various sensitive subgroups and Table \ref{tab:reduced-directory-structure} shows the metadata. 

\begin{table*}[]
\centering
\begin{tabular}{|p{3cm}|p{8cm}|}
\hline
\textbf{Hosp} & 
admissions.csv, diagnoses\_icd.csv, drgcodes.csv, labevents.csv, microbiologyevents.csv, omr.csv, pharmacy.csv, poe.csv, poe\_detail.csv, prescriptions.csv, procedures\_icd.csv, services.csv, transfers.csv \\
\hline
\textbf{ICU} & 
chartevents.csv, datetimeevents.csv, icustays.csv, ingredientevents.csv, inputevents.csv, outputevents.csv, procedureevents.csv \\
\hline
\textbf{ED} & 
diagnosis.csv, edstays.csv, medrecon.csv, pyxis.csv, triage.csv, vitalsign.csv \\
\hline
\textbf{CXR-JPG} & 
cxr\_chexpert.csv, cxr\_meta.csv, cxr\_negbio.csv, cxr\_split.csv \\
\hline
\textbf{CXR-DICOM} & 
s\{study\_id\}.txt \\
\hline
\textbf{REFLACX} & 
gaze.csv, anomaly\_location\_ellipses.csv, chest\_bounding\_box.csv, fixations.csv, timestamps\_transcription.csv, transcription.txt, metadata.csv \\
\hline
\textbf{EyeGaze} & 
audio\_segmentation\_transcripts/, bounding\_boxes.csv, eye\_gaze.csv, fixations.csv, master\_sheet.csv \\
\hline
\textbf{spreadsheets} & 
CXR-JPG/, cxr\_chexpert.csv, cxr\_negbio.csv, cxr\_split.csv, Hosp/, d\_hcpcs.csv, d\_icd\_diagnoses.csv, d\_icd\_procedures.csv, d\_labitems.csv, REFLACX/, metadata.csv, EyeGaze/, bounding\_boxes.csv, eye\_gaze.csv, fixations.csv, master\_sheet\_with\_updated\_stayId.csv, ICU/, d\_items.csv, cxr\_meta.csv, cxr\_meta\_with\_stay\_id\_only.csv \\
\hline
\end{tabular}
\caption{MIMIC-eye Directory Structure }
\label{tab:reduced-directory-structure}
\end{table*}

\section{Experimental Settings}
\label{apx:settings}
This section provides a detailed description of the various implementation decisions made during the entire ML model development pipeline and the experimental studies. The dataset is collated for each stayid and then the different modalities are encoded into the unified feature space as discussed in Section 3.1. We have sourced datasets from MIMIC Eye and MIMIC-IV ED. The dataset is randomly split into 80\% training(12501 stays) and 20\% testing subset(3126 stayids). For the ED Disposition task, we have used the Cross-Entropy Loss and the Binary Cross Entropy loss for the Multitask Binary Classification task. The Adam optimizer is used with a learning rate of 5e-5. The models were then trained on the training split on a CentOS 7.9.2009 system with 16GB of RAM and a NVIDIA V100-SXM2 GPU and experimental results were reported on the testing split. The training and the validation loss were kept track to train the model till the validation loss converged. The performance of the model on different evaluation metrics such as F1 score, AUROC, and AUPRC were also measured after every epoch. Since we have not observed any bias patterns in MIMIC-IV ED, we created a biased sampling as discussed in Section 5 and Table 6. 

\section{Modality-wise performance analysis: Multitask Learning}
\label{sec:multitask}
We conducted an extensive modality-wise performance comparison in multitask learning in Table \ref{tab:multitask_modality}. We have seen mixed performances across the modalities and the multimodal models. The F1 score for the multimodal model is comparatively high and the difference in performances for AUPRC and AUROC is negligible. We have chosen the multimodal model in the current study for multitask learning given the need to balance precision and recall in healthcare applications and are dealing with an imbalanced dataset where both false positives and false negatives are equally important.
\begin{table*}[]
    \centering
    \small
    \begin{tabular}{lccccccccc}
        \toprule
        \textbf{Modality} & \multicolumn{3}{c}{\textbf{Home}} & \multicolumn{3}{c}{\textbf{Mortality}} & \multicolumn{3}{c}{\textbf{ICU}} \\
        \cmidrule(lr){2-4} \cmidrule(lr){5-7} \cmidrule(lr){8-10}
        & \textbf{F1} & \textbf{AUROC} & \textbf{AUPRC} & \textbf{F1} & \textbf{AUROC} & \textbf{AUPRC} & \textbf{F1} & \textbf{AUROC} & \textbf{AUPRC} \\
        \midrule
        Arrival   & 0.151 & 0.451 & 0.509 & \textbf{0.064} & 0.515 & 0.039 & \textbf{0.371} & \textbf{0.563} & 0.269 \\
        Codes     & 0.253 & \textbf{0.521} & 0.548 & \textbf{0.064} & 0.485 & 0.032 & 0.367 & 0.495 & 0.219 \\
        Medrecon  & 0.563 & 0.503 & 0.549 & \textbf{0.064} & 0.489 & 0.032 & 0.370 & 0.528 & 0.259 \\
        Pyxis     & 0.632 & 0.496 & 0.549 & \textbf{0.064} & 0.522 & \textbf{0.042} & 0.369 & 0.493 & 0.222 \\
        Triage    & 0.082 & 0.473 & 0.527 & 0.063 & \textbf{0.525} & 0.038 & 0.367 & \textbf{0.563} & \textbf{0.289} \\
        Vitals    & 0.401 & 0.510 & 0.558 & 0.063 & 0.442 & 0.030 & 0.368 & 0.509 & 0.228 \\
        Xray      & 0.514 & 0.520 & \textbf{0.560} & \textbf{0.064} & 0.509 & 0.036 & 0.370 & 0.512 & 0.233 \\
        \midrule
        \textbf{Multimodal+events} & \textbf{0.705} & 0.503 & 0.549 & 0.063 & 0.452 & 0.036 & 0.370 & 0.487 & 0.226 \\
        \bottomrule
    \end{tabular}
    \caption{Performance Metrics for Different Modalities}
    \label{tab:multitask_modality}
\end{table*}
\section{Bias Analysis}

\textbf{Bias Analysis of MIMIC-IV ED}: In Table 5, we show the bias analysis on the ED disposition task for MIMIC-IV ED. It exhibits no DP, TPR, or WP disparity among the demographic groups and intersections.  

\textbf{Biased Sampling of MIMIC-IV ED}: For performing the bias mitigation using our proposed SDAE, a biased subset is constructed from the testing set of the MIMIC-IV-ED dataset. All the samples (100\%) from the privileged class (White Male and White Female) are taken. For the minority class (Non-White Male and Non-White Female), a fraction (50\%) of the true positive and true negative class instances are randomly sampled and added to our subset (Table \ref{tab:mimicbias}).
\begin{table*}[hbt!]
\centering
\small
\begin{tabular}{c|cc}
\toprule
\textbf{Group} & \multicolumn{2}{c}{\textbf{MIMIC-IV ED (original)}}  \\
% \cmidrule{2-5}
\midrule
 \textbf{Gender} & \textbf{DP} & \textbf{TPR} \\

Male (M) & 0.418 & 0.968  \\
Female (F) & 0.419 & 0.969  \\
\hline
\textbf{WP} &\cellcolor{green!30}0.997  &\cellcolor{green!30}0.998    \\
\hline
\textbf{Race}&& \\
White & 0.420 & 0.969 \\
Non-White & 0.415 & 0.968   \\
\hline
\textbf{WP} &\cellcolor{green!30}0.988  &\cellcolor{green!30}0.998    \\
\hline
\textbf{Race-Gender}&&\\
White-M & 0.420 & 0.969  \\
White-F & 0.421 & 0.969  \\
NonWhite-M & 0.414 & 0.965  \\
NonWhite-F & 0.416 & 0.970  \\
\hline
\textbf{WP} &\cellcolor{green!30}0.985  & \cellcolor{green!30}0.994  \\
\bottomrule
\end{tabular}
\caption{Performance metrics across different groups for the original MIMIC-IV ED. DP: Disparate Impact, TPR: True Positive Rate; WP:Worst case Parity.}
\label{tab:performance_metrics}
\end{table*}

\textbf{Multitask Bias Analysis of MIMIC-Eye}: In an extended analysis (Table \ref{tab:bias}) involving binary race categories and gender, there is no discrepancy in terms of WP on disposition, but white females and non-white females exhibit WP disparity(DP) in mortality prediction and all the groups except white males show WP(TPR) disparity.  and Asian males exhibit biases at home and in ICU predictions (TPR). Mortality and ICU predictions are the most biased among all tasks, where equity is paramount. 

\begin{table*}[hbt!]
    \centering
    \small
    \begin{tabular}{c|cccccc}
        \toprule
        \multicolumn{1}{c|}{} & \multicolumn{6}{c}{\textbf{Multitask}} \\
        \hline
        \textbf{Group} & \textbf{Home} &  & \textbf{Mortality} &  & \textbf{ICU} & \\
        \midrule
        \textbf{Gender} & DP & TPR & DP & TPR & DP & TPR \\
        Male (M) &  \cellcolor{orange!50}0.514 & \cellcolor{orange!50}0.543 & \cellcolor{orange!100}0.037 & \cellcolor{orange!50}0.542 & \cellcolor{orange!100}0.239 & \cellcolor{orange!50}0.530 \\
        Female (F) & \cellcolor{orange!50}0.570 & \cellcolor{orange!30}0.550 & \cellcolor{orange!100}0.028 & \cellcolor{orange!30}0.551 & \cellcolor{orange!100}0.216 & \cellcolor{orange!50}0.531 \\
        \textbf{WP} &  \cellcolor{green!30}0.901 & \cellcolor{green!30}0.987 & \cellcolor{yellow!30}0.756 & \cellcolor{green!30}0.983 & \cellcolor{green!30}0.903 & \cellcolor{green!30}0.998 \\
        \hline
        \textbf{Race-Gender} & & & & & & \\
        Nonwhite-F &  \cellcolor{orange!50}0.567 & \cellcolor{orange!50}0.532 & \cellcolor{orange!100}0.034 & \cellcolor{orange!150} 0.000 & \cellcolor{orange!100}0.199 & \cellcolor{orange!50}0.195 \\
        Nonwhite-M &  \cellcolor{orange!100}0.477 & \cellcolor{orange!100}0.491 & \cellcolor{orange!100}0.033 & \cellcolor{orange!150} 0.000 & \cellcolor{orange!100}0.258 & \cellcolor{orange!100}0.256 \\
        White-F &  \cellcolor{orange!50}0.573 & \cellcolor{orange!50}0.561 & \cellcolor{orange!100}0.024 & \cellcolor{orange!150}0.000 & \cellcolor{orange!100}0.227 & \cellcolor{orange!100}0.211 \\
        White-M & \cellcolor{orange!50}0.537 & \cellcolor{orange!50}0.574 & \cellcolor{orange!100}0.040 & \cellcolor{orange!100} 0.047 & \cellcolor{orange!100}0.227 & \cellcolor{orange!100}0.213 \\
        \textbf{WP} &  \cellcolor{green!30}0.832 & \cellcolor{green!30}0.855 & \cellcolor{orange!30}0.600 & \cellcolor{orange!150}0.000 & \cellcolor{yellow!50}0.771 & \cellcolor{yellow!50}0.761 \\
        \hline
        Asian-F &  \cellcolor{orange!30}0.500 & \cellcolor{orange!30}0.647 & \cellcolor{orange!100}0.118 & \cellcolor{orange!150}0.000 & \cellcolor{orange!100}0.235 & \cellcolor{orange!100}0.300 \\
        Asian-M &  \cellcolor{orange!100}0.379 & \cellcolor{orange!50}0.428 & \cellcolor{orange!100}0.069 & \cellcolor{orange!150}0.000 & \cellcolor{orange!100}0.344 & \cellcolor{orange!100}0.166 \\
        Black-F &  \cellcolor{orange!30}0.606 & \cellcolor{orange!50}0.546 & \cellcolor{orange!100}0.031 & \cellcolor{orange!150}0.000 & \cellcolor{orange!100}0.166 & \cellcolor{orange!100}0.195 \\
        Black-M &  \cellcolor{orange!50}0.435 & \cellcolor{orange!30}0.428 & \cellcolor{orange!100}0.021 & \cellcolor{orange!150}0.000 & \cellcolor{orange!100}0.186 & \cellcolor{orange!100}0.200 \\
        White-F & \cellcolor{orange!30}0.573 & \cellcolor{orange!30}0.561 & \cellcolor{orange!100}0.024 & \cellcolor{orange!150}0.000 & \cellcolor{orange!100}0.227 & \cellcolor{orange!100}0.211 \\
        White-M & \cellcolor{orange!30}0.537 & \cellcolor{orange!30}0.574 & \cellcolor{orange!100}0.040 & \cellcolor{orange!100}0.047 & \cellcolor{orange!100}0.227 & \cellcolor{orange!100}0.213 \\
        \textbf{WP} & \cellcolor{orange!30}0.625 & \cellcolor{orange!30}0.661 & \cellcolor{orange!100}0.177 & \cellcolor{orange!150}0.000 & \cellcolor{orange!50}0.482 & \cellcolor{orange!50}0.553 \\
        \bottomrule
    \end{tabular}
    \caption{Evaluation of model biases with demographic intersections in MIMIC-Eye (color coding indicates the intensity of unfairness, where green indicates fair, orange indicates unfair, and yellow denotes medium fair)}
    \label{tab:bias}
\end{table*}

\section{Bias mitigation - Multitask Settings}
\label{ap:multitask}
We conduct an extensive bias analysis in a multitask binary setting and compare the performance across the base classifier, ROC enforced on gender, race, and the combination, and our proposed SDAE. The ROC-enforced models showed the same results which we denoted as $\mathcal M^{ROC}$. The comparison is given in Figures \ref{fig:mortality1}, \ref{fig:icu1}, and  \ref{fig:home1}. Our proposed SDAE shows consistent improvement in the three multitask settings without injecting additional biases into other subgroups. 
\begin{figure*}[hbt!]
    \centering
    
    \begin{subfigure}[b]{0.45\textwidth}
        \centering
        \includegraphics[width=\textwidth]{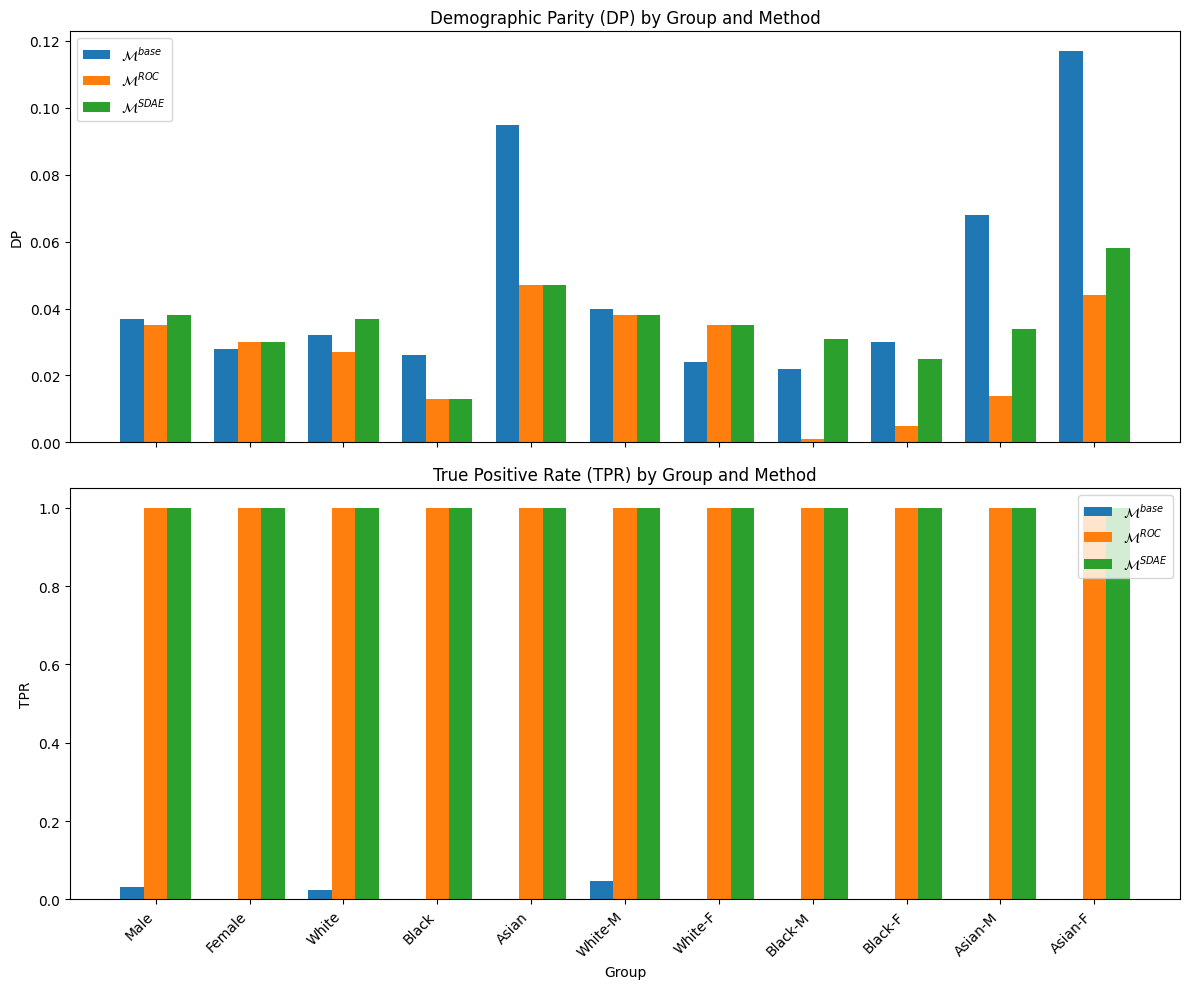}
        \caption{Mortality}
        \label{fig:mortality1}
    \end{subfigure}
    \hfill
    \begin{subfigure}[b]{0.45\textwidth}
        \centering
        \includegraphics[width=\textwidth]{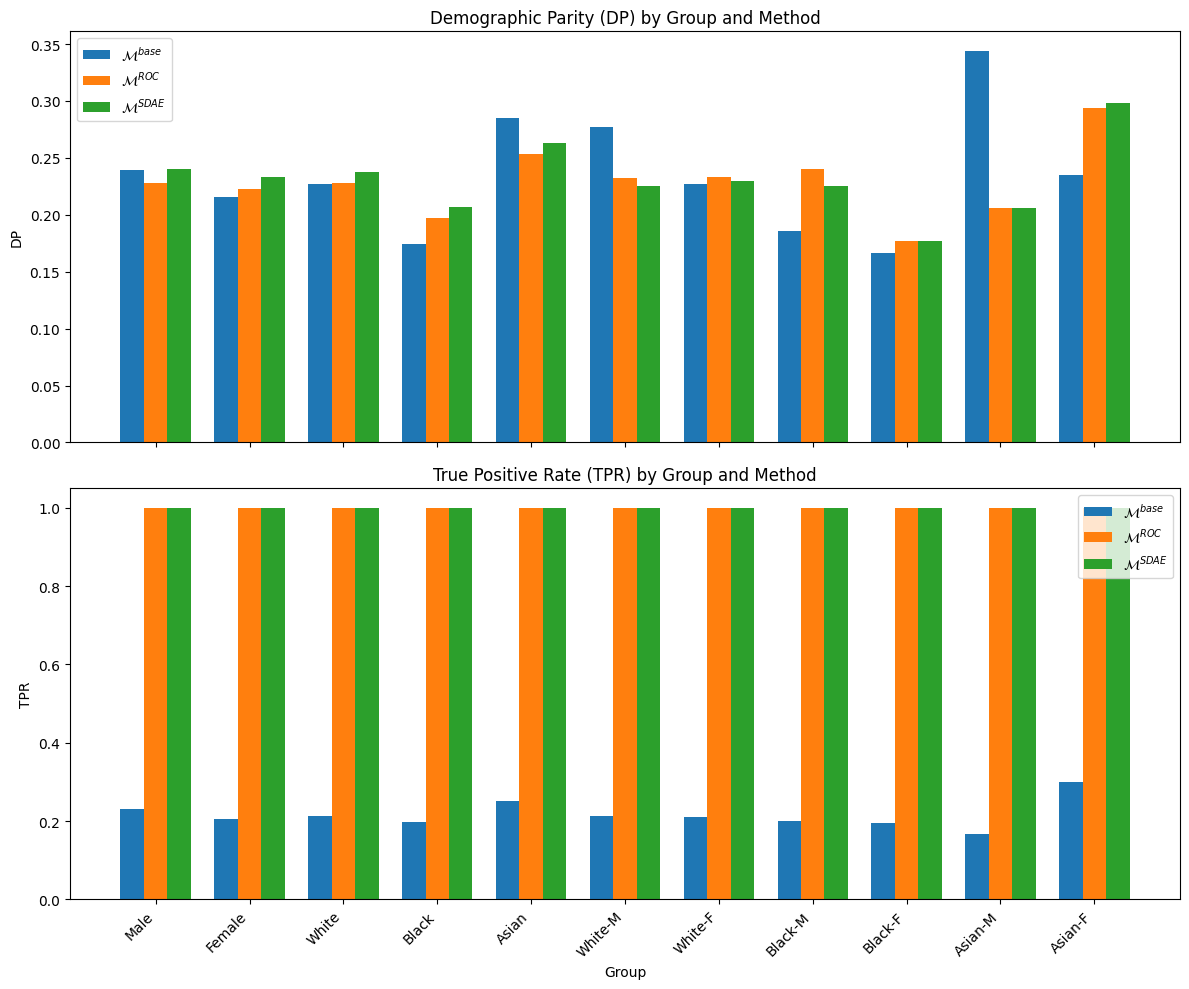}
        \caption{ICU}
        \label{fig:icu1}
    \end{subfigure}
    \hfill
    \begin{subfigure}[b]{0.45\textwidth}
        \centering
        \includegraphics[width=\textwidth]{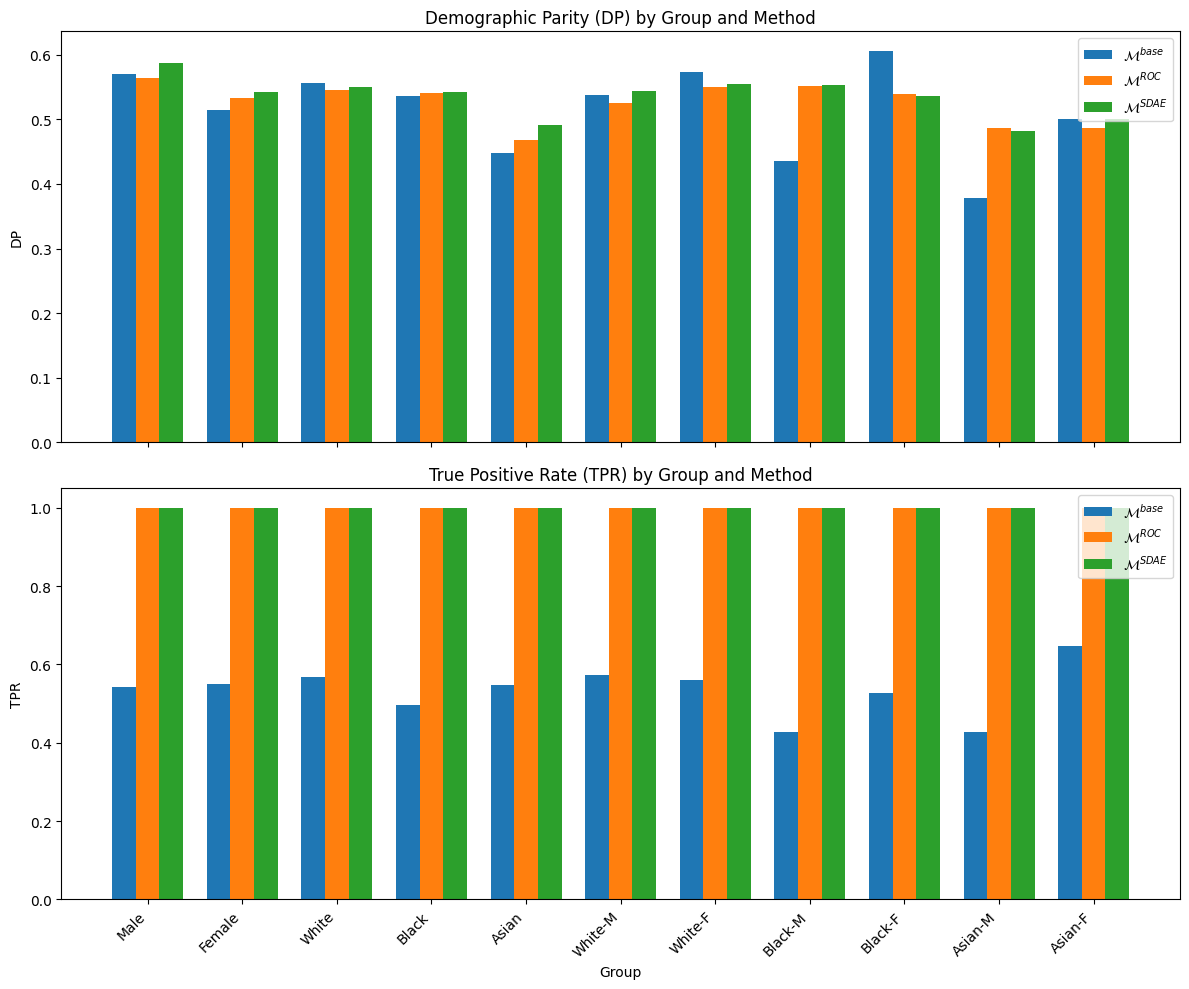}
        \caption{Home}
        \label{fig:home1}
    \end{subfigure}
    
    \caption{Comparison of Worstcase Parity (WP) in multitask learning across the subgroups}
    \label{fig:overall_label1}
\end{figure*}

\begin{table*}[hbt!]
\centering
\small
\begin{tabular}{cccc}
\toprule
\textbf{Gender} & \multicolumn{2}{c|}{\textbf{Race}} & \textbf{Total} \\
% \cmidrule{2-3}
 & \textbf{White} & \textbf{Non-White} & \\
\midrule
Male &  33862(35.16\%) &  11008(11.43\%) &  44870(46.59\%) \\
Female &  35245(37.64\%) & 15185(15.77\%) &  51430(53.41\%)  \\

\textbf{Total} &  70107(72.80\%) &  26193(27.20\%) &  96300(100\%) \\
\bottomrule
\end{tabular}
\caption{Distribution of Stay IDs and subgroup statistics in the biased sample of MIMIC-IV-ED}
\label{tab:mimicbias}
\end{table*}

\end{document}
